# Supplementary material for: Sequential Bayesian Learning for Hidden Semi-Markov Models
Source: arXiv:2301.10494 source file (2023-01-25)
Supplement: Supplementary file 1 [file Appendix_Models.tex]

%%%%%%%%%%%%%%%%%%%%%%%%%%%%%%%%%%%%%%%%%%%%%%%%%%%%%%%%%%%%%%%%%%%%%%%%%
%%%%%%%%%%%%%%%%%%%%%%%%%%%%%%%%%%%%%%%%%%%%%%%%%%%%%%%%%%%%%%%%%%%%%%%%%
%%%%%%%%%%%%%%%%%%%%%%%%%%%%%%%%%%%%%%%%%%%%%%%%%%%%%%%%%%%%%%%%%%%%%%%%%
\section{Model distributions and prior assumptions} \label{sec:App_ModelDistributions}

%%%%%%%%%%%%%%%%%%%%%%%%%%%%%%%%%%%%%%%%%%%%%%%%%%%%%%%%%%%%%%%%%%%%%%%%%
\subsection{Models used in section \ref{sec:Experiments}}

\begin{itemize}
    \item \textbf{HSMM with Negative Binomial duration},  \newline
    Model parameter: $\theta = \{\mu, \sigma, k, r, p \}$.
    \begin{itemize}
        \item Model dynamics:
    	\begin{itemize} 
    	    \item Data $E_t \sim N(\mu_{s_t}, \sigma_{s_t})$, 
    	    \item Latent state $S_t \sim  \begin{cases} %\mid \{ S_{t-1} = s_{t-1}, D_{t-1} = d_{t-1} \} 
            \delta( s_{t}, s_{t-1}) &\text{ $d_{t-1} > 0$ }\\
            Categorical(k_{s_{t-1}}) &\text{ $d_{t-1} = 0$ }
            \end{cases}$,
            \item Latent duration $D_t \sim \begin{cases} %\mid \{ S_{t} = s_{t}, D_{t-1} = d_{t-1} \} 
            \delta( d_{t}, d_{t-1} - 1) &\text{ $d_{t-1} > 0$ }\\
            NegativeBinomial(r_{s_{t}}, p_{s_{t}}) &\text{ $d_{t-1} = 0$ }
            \end{cases}$,
        \end{itemize}
        \item Model parameter priors:
        \begin{itemize}
            \item $\mu_1 \sim Normal_{(-100, 0)}(\mu = -2, \sigma = 10^5)$,
            \item $\mu_2 \sim Normal_{(0, 100)}(\mu = 2, \sigma = 10^5)$,
            \item $\sigma \sim Normal_{(0, 10)}(\mu = 2, \sigma = 10^5)$,
            \item $r \sim Normal_{(0, 100]}(\mu = 10, \sigma = 10^5)$,
            \item $p \sim Beta(\alpha = 1, \beta = 1)$,
            \item $k \sim Dirichlet( \alpha_1 = \alpha_2 = ... = \alpha_k = k),$ where $k =$ number of latent states.
        \end{itemize}
    \end{itemize}
\end{itemize}
        
%%%%%%%%%%%%%%%%%%%%%%%%%%%%%%%%%%%%%%%%%%%%%%%%%%%%%%%%%%%%%%%%%%%%%%%%%        
\subsection{Models used in section \ref{sec:ApplicationsVIX}}
\begin{itemize}
    \item \textbf{AR(1) HSMM with Negative Binomial duration},  \newline
    Model parameter: $\theta = \{\mu, \sigma, w, k, r, p \}$.
    \begin{itemize}
        \item Model dynamics:
    	\begin{itemize} 
    	    \item Data $E_t \sim N(w_{s_t} \times e_{t-1} + \mu_{s_t}, \sigma_{s_t})$, 
    	    \item Latent state $S_t \sim  \begin{cases} %\mid \{ S_{t-1} = s_{t-1}, D_{t-1} = d_{t-1} \} 
            \delta( s_{t}, s_{t-1}) &\text{ $d_{t-1} > 0$ }\\
            Categorical(k_{s_{t-1}}) &\text{ $d_{t-1} = 0$ }
            \end{cases}$,
            \item Latent duration $D_t \sim \begin{cases} %\mid \{ S_{t} = s_{t}, D_{t-1} = d_{t-1} \} 
            \delta( d_{t}, d_{t-1} - 1) &\text{ $d_{t-1} > 0$ }\\
            NegativeBinomial(r_{s_{t}}, p_{s_{t}}) &\text{ $d_{t-1} = 0$ }
            \end{cases}$,
        \end{itemize}
        \item Model parameter priors:
        \begin{itemize}
            \item $\mu \sim Normal_{(0, 10)}(\mu = 2, \sigma = 10^5)$,
            \item $\sigma \sim Normal_{(0, 10)}(\mu = 0.01, \sigma = 10^5)$,
            \item $w \sim Normal_{(-1, 1)}(\mu = 0, \sigma = 10^5)$,
            \item $r \sim Normal_{(0, 100]}(\mu = 20, \sigma = 10^5)$,
            \item $p \sim Beta(\alpha = 1, \beta = 1)$,
            \item $k \sim Dirichlet( \alpha_1 = \alpha_2 = ... = \alpha_k = k),$ where $k =$ number of latent states.
        \end{itemize}
    \end{itemize}
    
    \item \textbf{AR(1) HSMM with Poisson duration},  \newline
    Model parameter: $\theta = \{\mu, \sigma, w, k, \lambda \}$.
    \begin{itemize}
        \item Model dynamics:
    	\begin{itemize} 
    	    \item Data $E_t \sim N(w_{s_t} \times e_{t-1} + \mu_{s_t}, \sigma_{s_t})$, 
    	    \item Latent state $S_t \sim  \begin{cases} %\mid \{ S_{t-1} = s_{t-1}, D_{t-1} = d_{t-1} \} 
            \delta( s_{t}, s_{t-1}) &\text{ $d_{t-1} > 0$ }\\
            Categorical(k_{s_{t-1}}) &\text{ $d_{t-1} = 0$ }
            \end{cases}$,
            \item Latent duration $D_t \sim \begin{cases} %\mid \{ S_{t} = s_{t}, D_{t-1} = d_{t-1} \} 
            \delta( d_{t}, d_{t-1} - 1) &\text{ $d_{t-1} > 0$ }\\
            Poisson(\lambda_{s_{t}}) &\text{ $d_{t-1} = 0$ }
            \end{cases}$,
        \end{itemize}
        \item Model parameter priors:
        \begin{itemize}
            \item $\mu \sim Normal_{(0, 10)}(\mu = 2, \sigma = 10^5)$,
            \item $\sigma \sim Normal_{(0, 10)}(\mu = 0.01, \sigma = 10^5)$,
            \item $w \sim Normal_{(-1, 1)}(\mu = 0, \sigma = 10^5)$,
            \item $\lambda \sim Normal_{(0, 100]}(\mu = 20, \sigma = 10^5)$,
            \item $k \sim Dirichlet( \alpha_1 = \alpha_2 = ... = \alpha_k = k),$ where $k =$ number of latent states.
        \end{itemize}
    \end{itemize}

    \item \textbf{AR(1) HMM},  \newline
    Model parameter: $\theta = \{\mu, \sigma, w, k \}$.
    \begin{itemize}
        \item Model dynamics:
    	\begin{itemize} 
    	    \item Data $E_t \sim N(w_{s_t} \times e_{t-1} + \mu_{s_t}, \sigma_{s_t})$, 
    	    \item Latent state $S_t \sim Categorical(k_{s_{t-1}})$,
        \end{itemize}
        \item Model parameter priors:
        \begin{itemize}
            \item $\mu \sim Normal_{(0, 10)}(\mu = 2, \sigma = 10^5)$,
            \item $\sigma \sim Normal_{(0, 10)}(\mu = 0.01, \sigma = 10^5)$,
            \item $w \sim Normal_{(-1, 1)}(\mu = 0, \sigma = 10^5)$,
            \item $k \sim Dirichlet( \alpha_1 = \alpha_2 = ... = \alpha_k = k),$ where $k =$ number of latent states.
        \end{itemize}
    \end{itemize}
    
    \item \textbf{AR(1) Model}, \newline
    Model parameter: $\theta = \{\mu, \sigma, w \}$:
    \begin{itemize}
        \item Model dynamics:
    	\begin{itemize} 
	        \item Data $E_t \sim Normal(w \times e_{t-1} + \mu, \sigma)$,
        \end{itemize}
        \item Model parameter priors:
        \begin{itemize}
            \item $\mu \sim Normal(\mu = 0, \sigma = 10^5)$,
            \item $\sigma \sim Normal_{(0, 10]}(\mu = 2, \sigma = 10^5)$,
            \item $w \sim Normal_{(-1, 1)}(\mu = 0, \sigma = 10^5)$.
        \end{itemize}
    \end{itemize}    
    
\end{itemize}
